# Supplementary material for: TGIF: A New Dataset and Benchmark on Animated GIF Description
Source: arXiv:1604.02748 source file (2016-04-12)
Supplement: Supplementary file 1 [file p1672-supp-r.pdf]

## Supplementary Material for *TGIF: A New Dataset and Benchmark on Animated GIF Description*

Yuncheng Li  
University of Rochester

Yale Song  
Yahoo Research

Liangliang Cao  
Yahoo Research

Joel Tetreault  
Yahoo Research

Larry Goldberg  
Yahoo Research

Alejandro Jaimes  
AiCure

Jiebo Luo  
University of Rochester

This supplementary material contains detailed information about the paper, specifically:

- Figure 1: A full version of the instructions shown to the crowd workers in reference to Section 3.2. Data Annotation).
- Figure 2: The task page shown to the workers (in reference to Section 3.2. Data Annotation).
- Figure 3: Syntactic validation error messages shown to the workers (In reference to Section 3.2).
- Figure 4: Example animated GIFs with generated descriptions (in reference to Section 5.3 Results and Discussion).
- Figure 5: Side-by-side qualitative comparisons of sentences provided in the LSMDC dataset (professionally annotated descriptive video service (DVS) captions) and sentences annotated by the crowd workers (in reference to Section 2.1. Comparison with LSMDC).

In Figure 4 and Figure 5, we provide one still frame of each animated GIF for easy visualization. However, the still frames are inadequate for showing the dynamic visual content of animated GIFs. We therefore invite the reviewers to the following websites as an alternative to Figure 4 and Figure 5. Each website also contains more examples than we provide in this supplementary material.

- Figure 4: <https://goo.gl/xCYjjE>
- Figure 5: <https://goo.gl/ZGYIYh>

## Instructions

### Task

Below you will see five animated GIFs. Your task is to describe each animated GIF in one English sentence. You should focus solely on the **visual content** presented in the animated GIF. Each sentence should be grammatically correct. It should describe the main characters and their actions, but NOT your opinions, guesses or interpretations.

### DOs

- Please use only English words. No digits allowed (spell them out, e.g., three).
- Each sentence must contain between 8 and 25 words. Try to be concise.
- Each sentence must contain a verb.
- If possible, include adjectives that describe colors, size, emotions, or quantity.
- Please pay attention to grammar and spelling.
- Each sentence must express a complete idea, and make sense by itself.
- The sentence should describe the main characters, actions, setting, and relationship between the objects.

### DON'Ts

- The sentence should NOT contain any digits.
- The sentence should NOT mention the name of a movie, film, and character.
- The sentence should NOT mention invisible objects and actions.
- The sentence should NOT make subjective judgments about the GIF.
- The sentence should NOT contain "there is" phrases, such as "there is", "there are", or "there exist"

Remember, please describe only the visual content presented in the animated GIF. Focus on the main characters and their actions.

### Examples

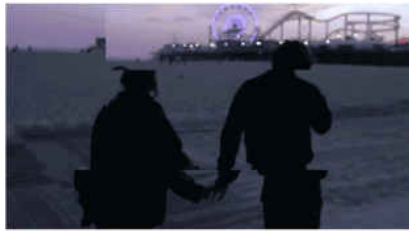

#### Acceptable descriptions

- Two lovers holding hands are walking near the beach.
- A couple holding hands is walking on a beach near an amusement park pier.

#### Unacceptable descriptions

- Felicity and Anton being lovebirds in movie Like Crazy. -- mentioning movie name and the character names
- Be happy, do not worry for nothing, blesses. -- subjective judgments/comments, slightly ungrammatical
- Couples are walking away from the camera. -- mentioning invisible objects: camera

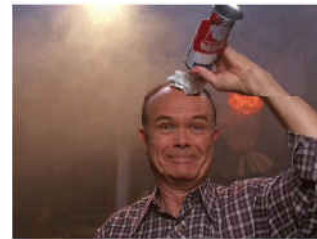

#### Acceptable descriptions

- A bald man is holding whipped cream over his head.
- A man wearing a plaid shirt is spraying whipped cream on his head.

#### Unacceptable descriptions

- I love this GIF. -- too short (4 words only) and not describing the animated GIF.
- A hot guy is funny. -- too short and not describing the animated GIF.
- Someone is looking forward. -- too short, and does not describe the main action the man is performing
- Someone is in a dark theater. -- does not describe the main character, nor the main action.
- Man and cream -- not a complete sentence.
- Funny, loved this GIF. -- mentioning about something, does not describe visible actions in the animated GIF.

Figure 1: A full version of the instructions shown to the crowd workers.

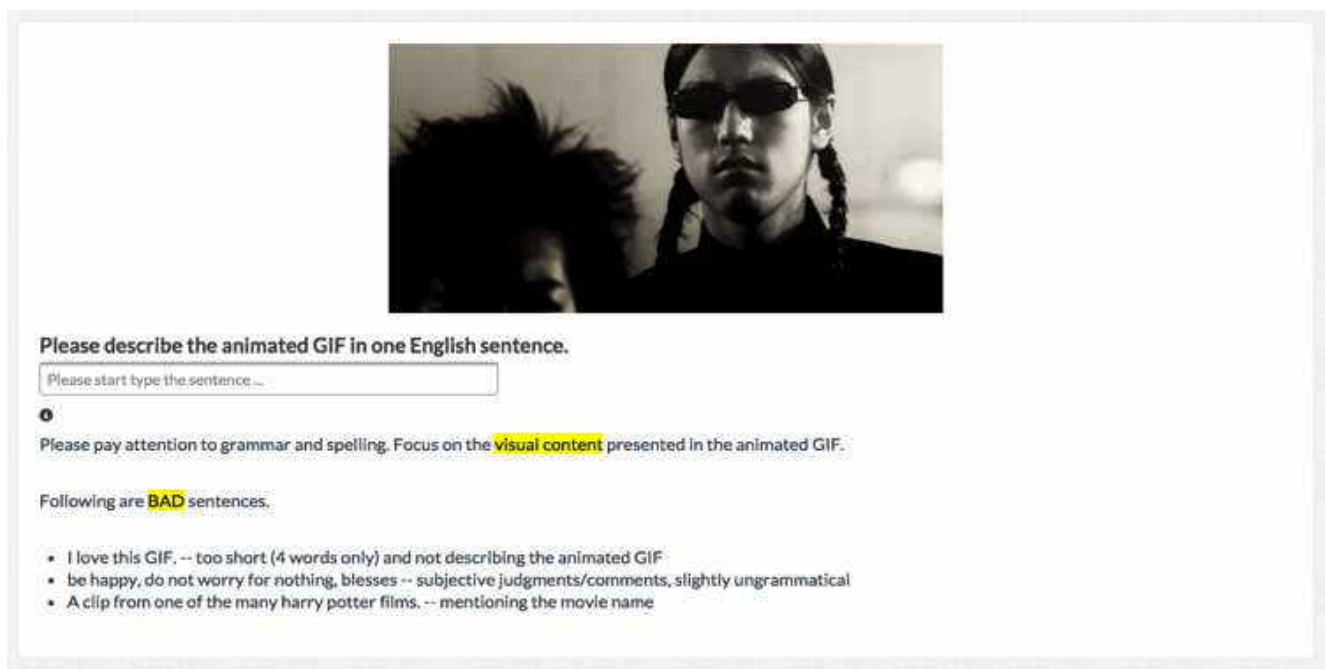

Please describe the animated GIF in one English sentence.

Please start type the sentence ...

Please pay attention to grammar and spelling. Focus on the **visual content** presented in the animated GIF.

Following are **BAD** sentences.

- I love this GIF. -- too short (4 words only) and not describing the animated GIF
- be happy, do not worry for nothing, blesses -- subjective judgments/comments, slightly ungrammatical
- A clip from one of the many harry potter films. -- mentioning the movie name

Figure 2: **Task page.** Each task page showed 5 animated GIFs and asked the worker to describe each with one sentence. This figure shows one of the five questions in a task page.

Please describe the animated GIF in one English sentence.

validation failed

Please start type the sentence ...

The sentence is too short. (digits are not counted)

(a) A sentence must contain at least 8, but no more than 25 words.

Please describe the animated GIF in one English sentence.

validation failed

两个人在对视

English words only.

(b) A sentence must contain only English words.

Please describe the animated GIF in one English sentence.

validation failed

Two people, one with long hair and the other with mask

Ungrammatical sentence. A grammatical sentence should have a subject, verb and object. Please refer to the instructions for acceptable sentences. Examples of Ungrammatical sentences,  
A female gymnast on the uneven bars.  
Someone coming into the house, carrying his skateboard. (Correction: Someone came into the house, carrying his skateboard.)

(c) A sentence must contain a main verb.

Please describe the animated GIF in one English sentence.

validation failed

A man is glaring, and someone with sunglasses appears

Line 1, column 47, Rule ID: MORFOLOGIK\_RULE\_EN\_US  
Message: Possible spelling mistake found  
Suggestion: appears; pairs; piers; Spears; spears; pears; spares; amperes; pares; apexes; rapiers; a pears  
...is glaring, and someone with sunglasses appears  
\*\*\*\*\*

(d) A sentence must be grammatical and free of typos.

Please describe the animated GIF in one English sentence.

validation failed

A man is glaring, and someone with sunglasses is is appearing

Line 1, column 47, Rule ID: ENGLISH\_WORD\_REPEAT\_RULE  
Message: Possible typo: you repeated a word  
Suggestion: is  
...is glaring, and someone with sunglasses is is appearing  
\*\*\*\*\*  
Line 1, column 50, Rule ID: PROGRESSIVE\_VERBS[1]  
Message: This verb is normally not used in the progressive form. Try a simple form instead.  
...glaring, and someone with sunglasses is is appearing  
\*\*\*\*\*

(e) A sentence must be grammatical and free of typos.

Please describe the animated GIF in one English sentence.

validation failed

A man is glaring, and Jordan with sunglass appears

Names such as "Jordan" should not be mentioned

(f) A sentence must contain no named entities, such as an actor/actress, movie names, countries.

Figure 3: **Syntactic validation.** Since the workers provide free-form text, we validate the sentence before submission to reduce syntactic errors. This figure shows example messages shown to the workers in case we detect a syntactic error: error type (red speech balloon) and explanation for the error (caption below text input).

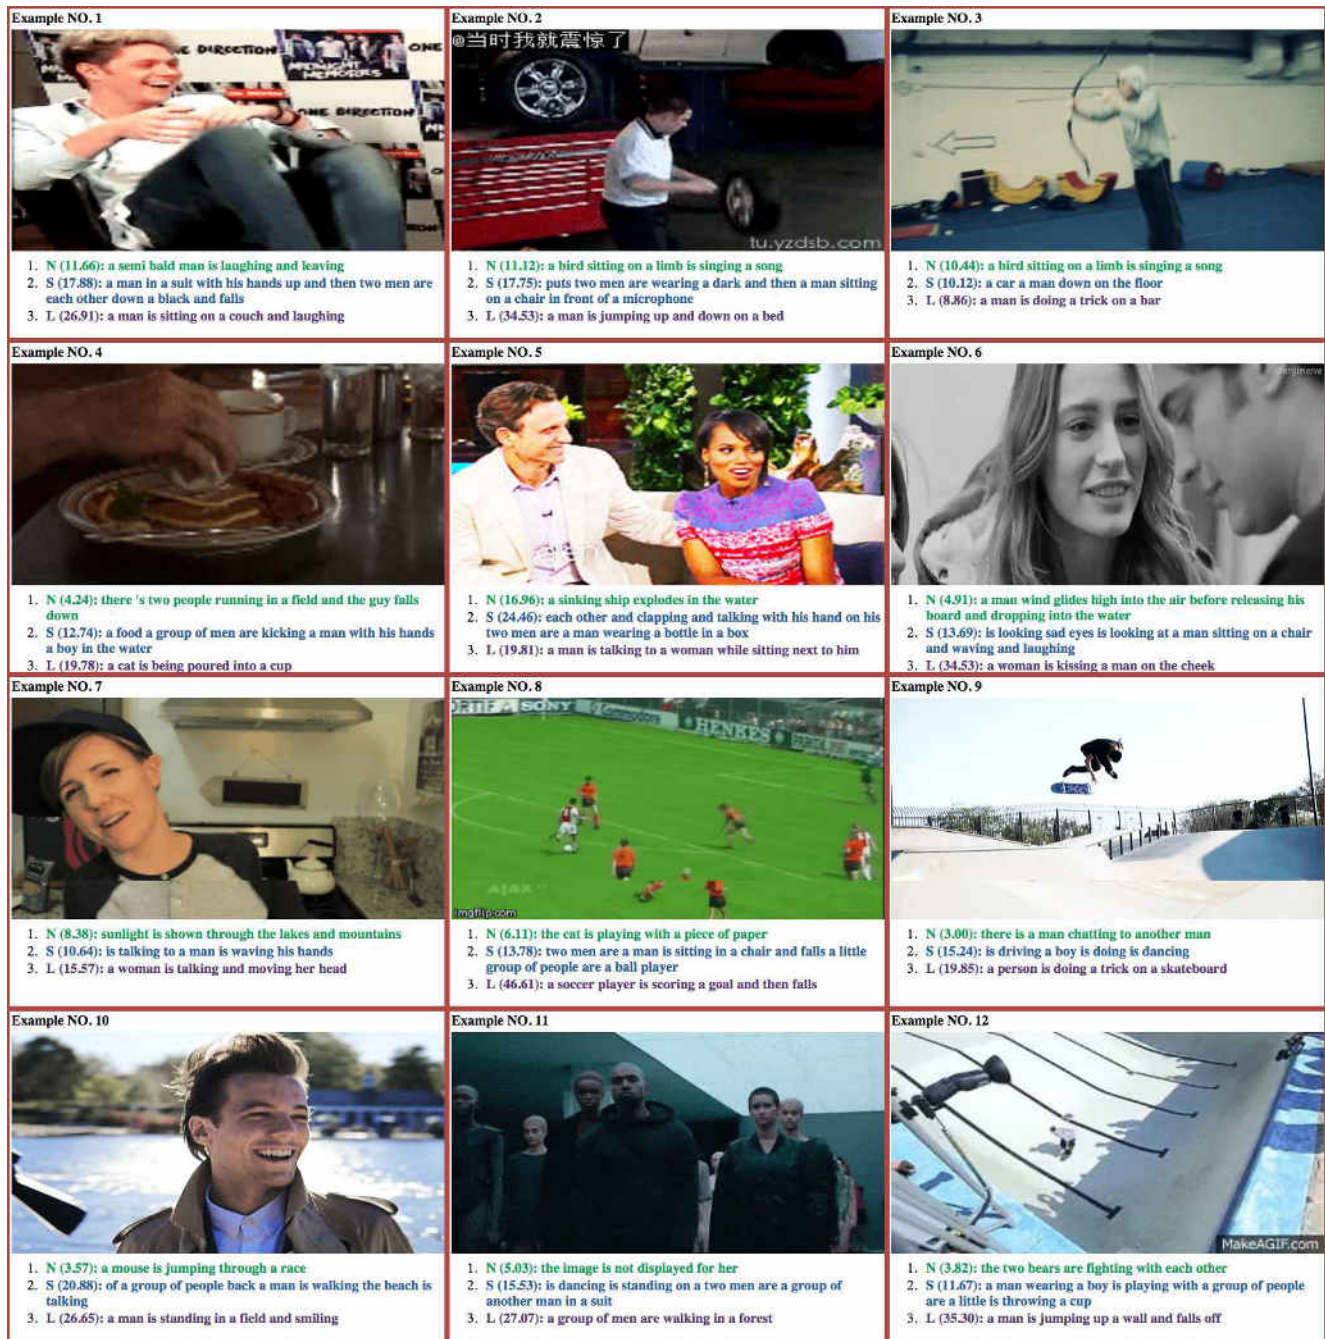

Figure 4: **Example animated GIFs and sentences generated** using the following algorithms: **nearest neighbor (N)**, **SMT-FrameNet (S)**, and **LSTM-Finetune (L)**. The numbers in parentheses show the METEOR score (%) of each generated sentence. More examples with better visualization: <https://goo.gl/xoYjjE>

|                                                                                                                                                                                                                                                                                                    |                                                                                                                                                                                                                                                            |                                                                                                                                                                                                                                                                                                     |
|----------------------------------------------------------------------------------------------------------------------------------------------------------------------------------------------------------------------------------------------------------------------------------------------------|------------------------------------------------------------------------------------------------------------------------------------------------------------------------------------------------------------------------------------------------------------|-----------------------------------------------------------------------------------------------------------------------------------------------------------------------------------------------------------------------------------------------------------------------------------------------------|
| <p>Example NO. 1</p> 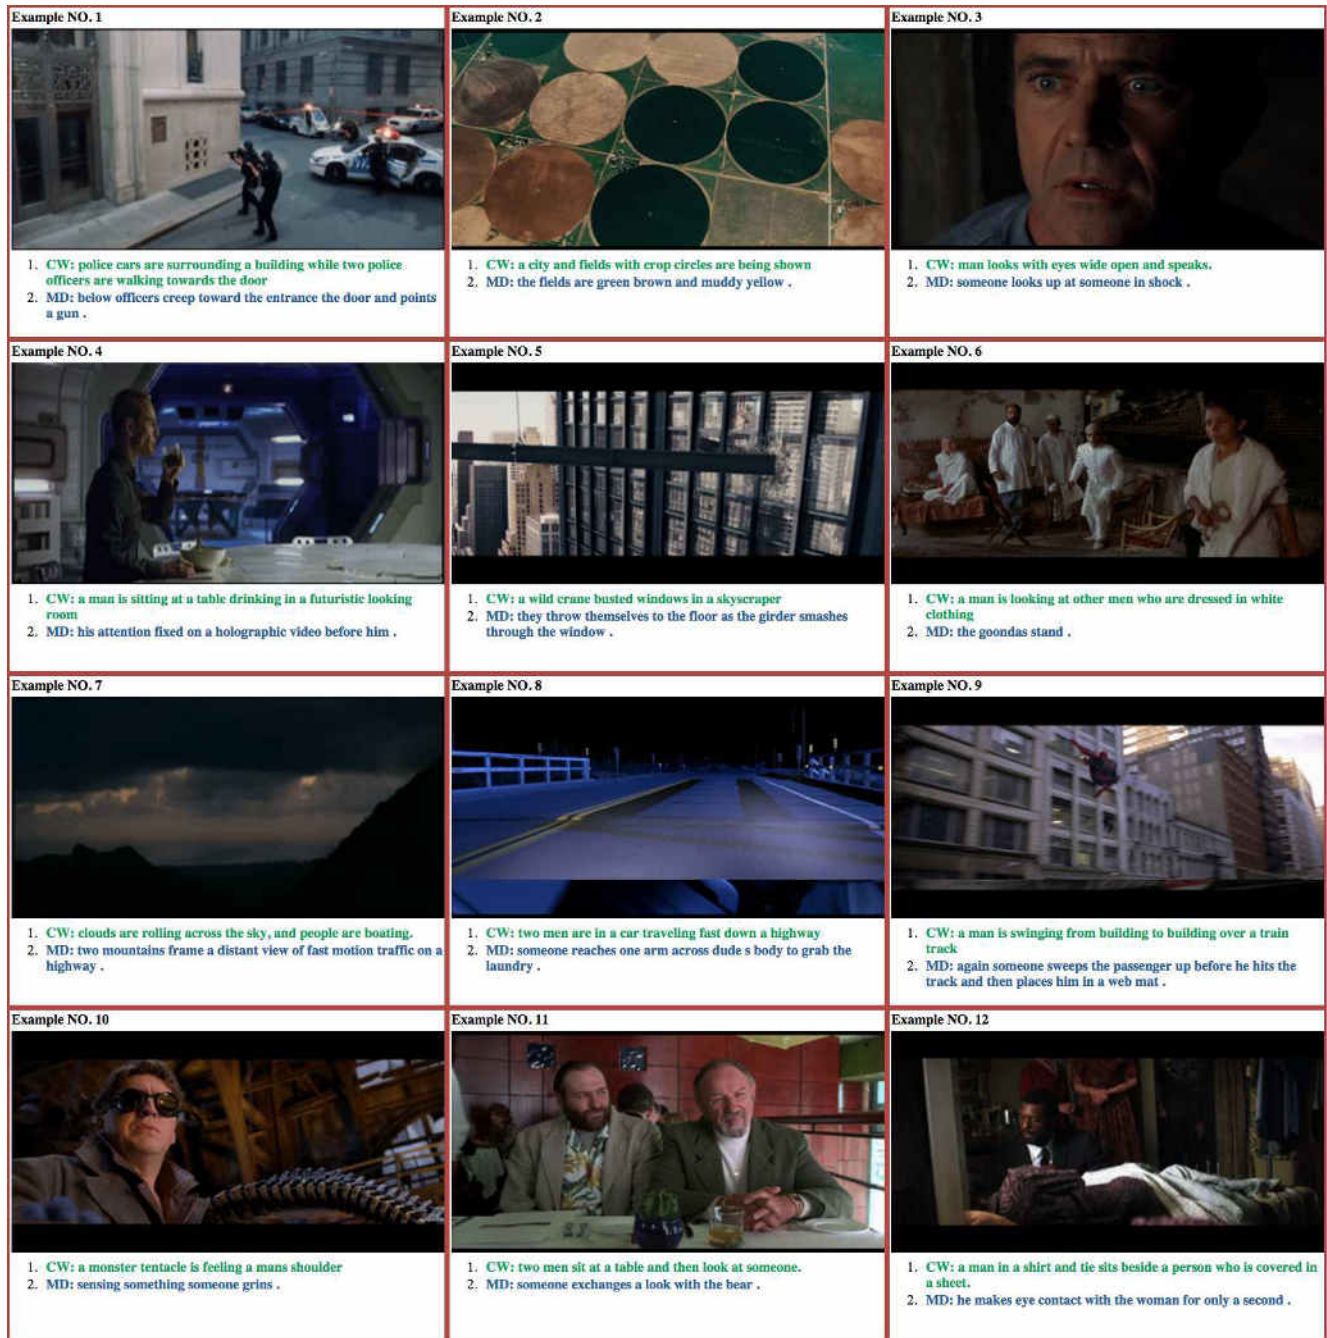 <p>1. CW: police cars are surrounding a building while two police officers are walking towards the door<br/>2. MD: below officers creep toward the entrance the door and points a gun .</p> | <p>Example NO. 2</p> 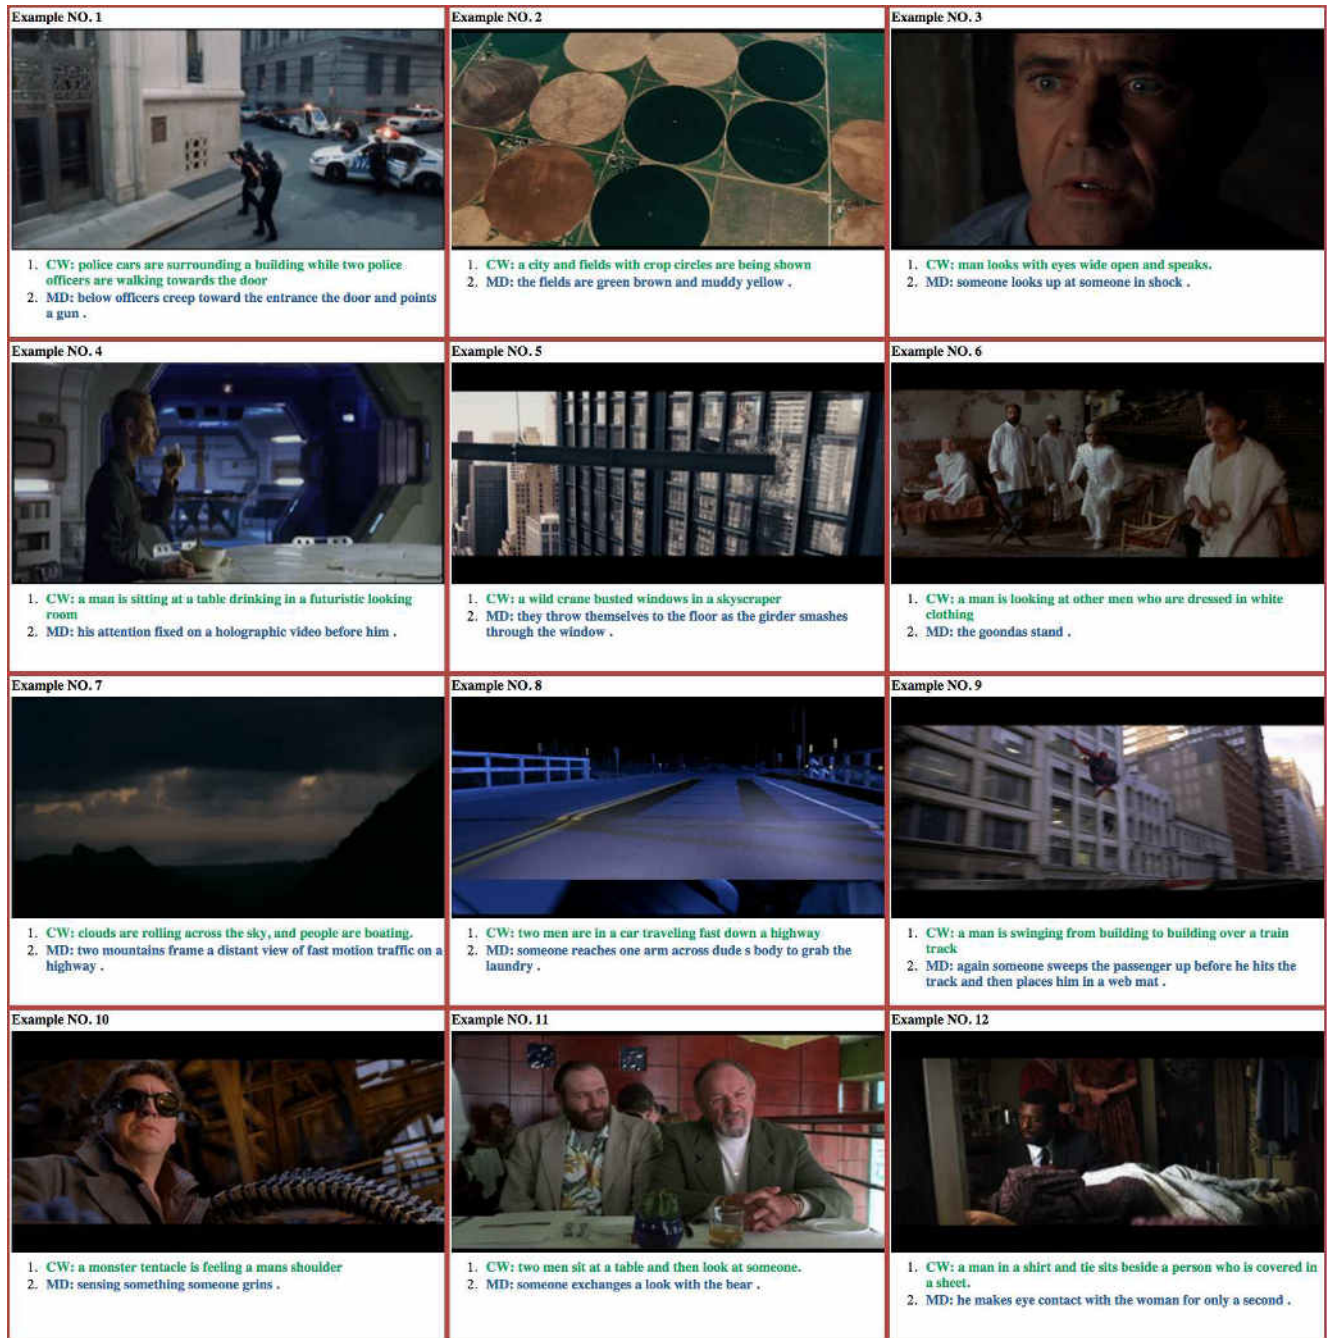 <p>1. CW: a city and fields with crop circles are being shown<br/>2. MD: the fields are green brown and muddy yellow .</p>                         | <p>Example NO. 3</p> 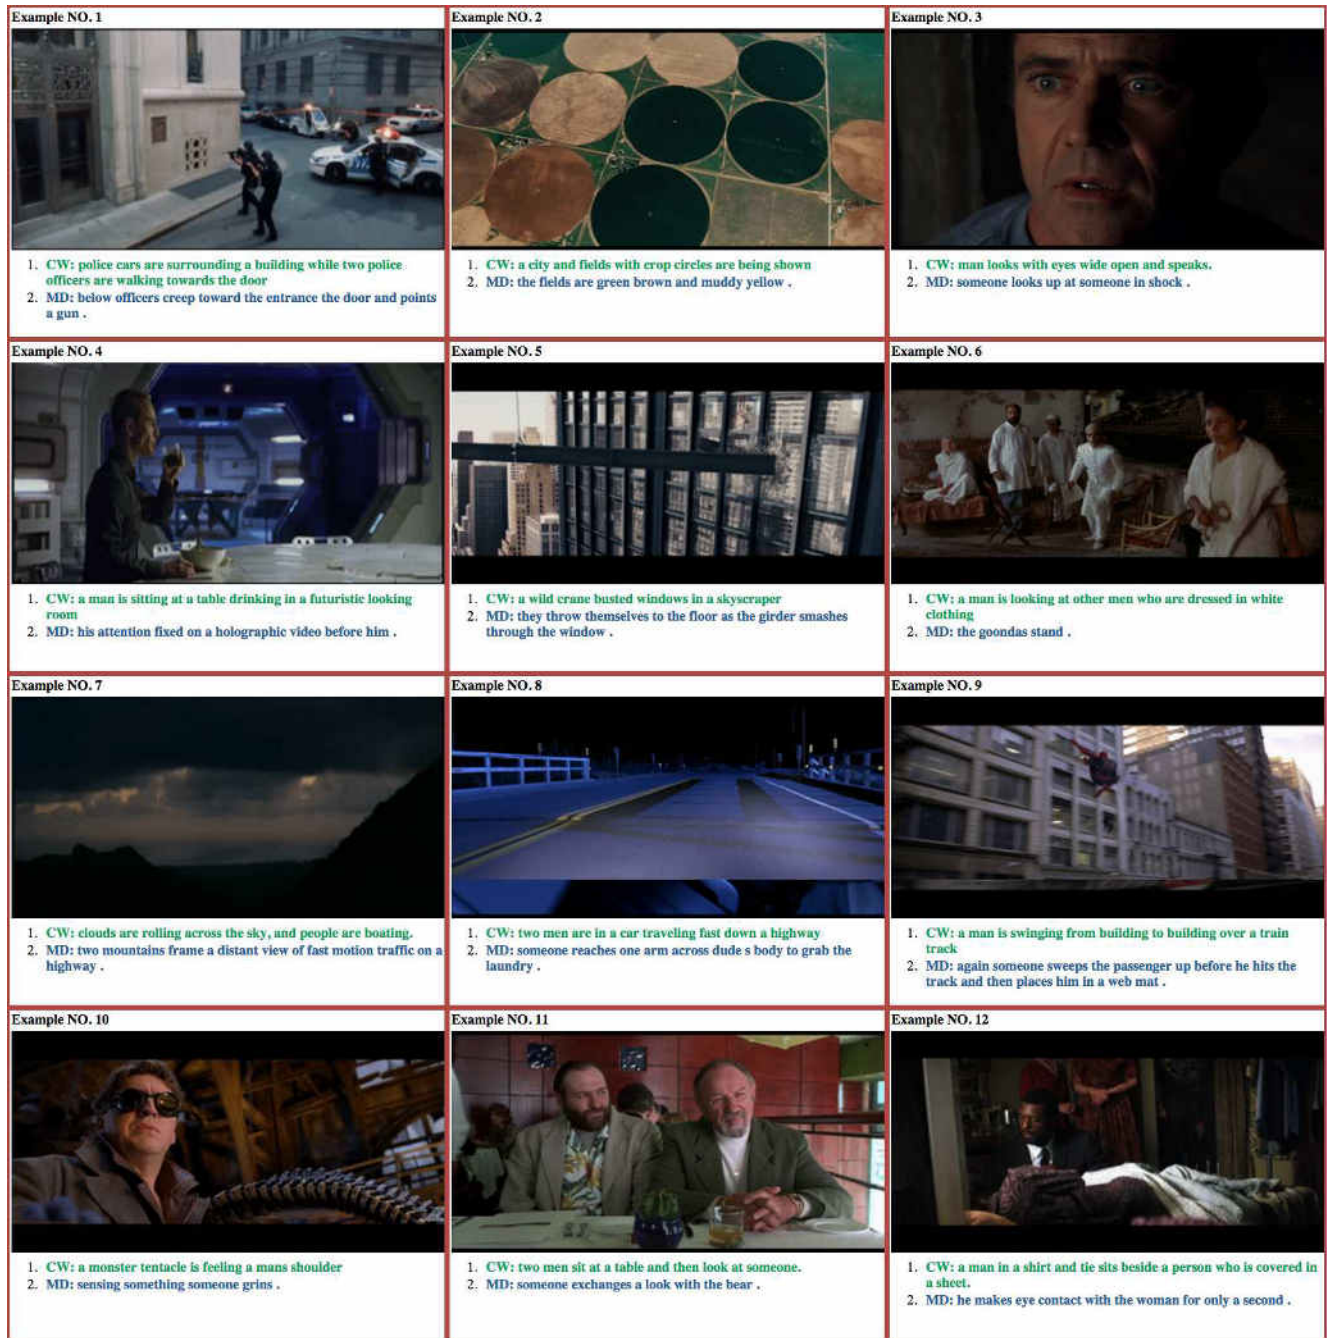 <p>1. CW: man looks with eyes wide open and speaks.<br/>2. MD: someone looks up at someone in shock .</p>                                                                                  |
| <p>Example NO. 4</p> 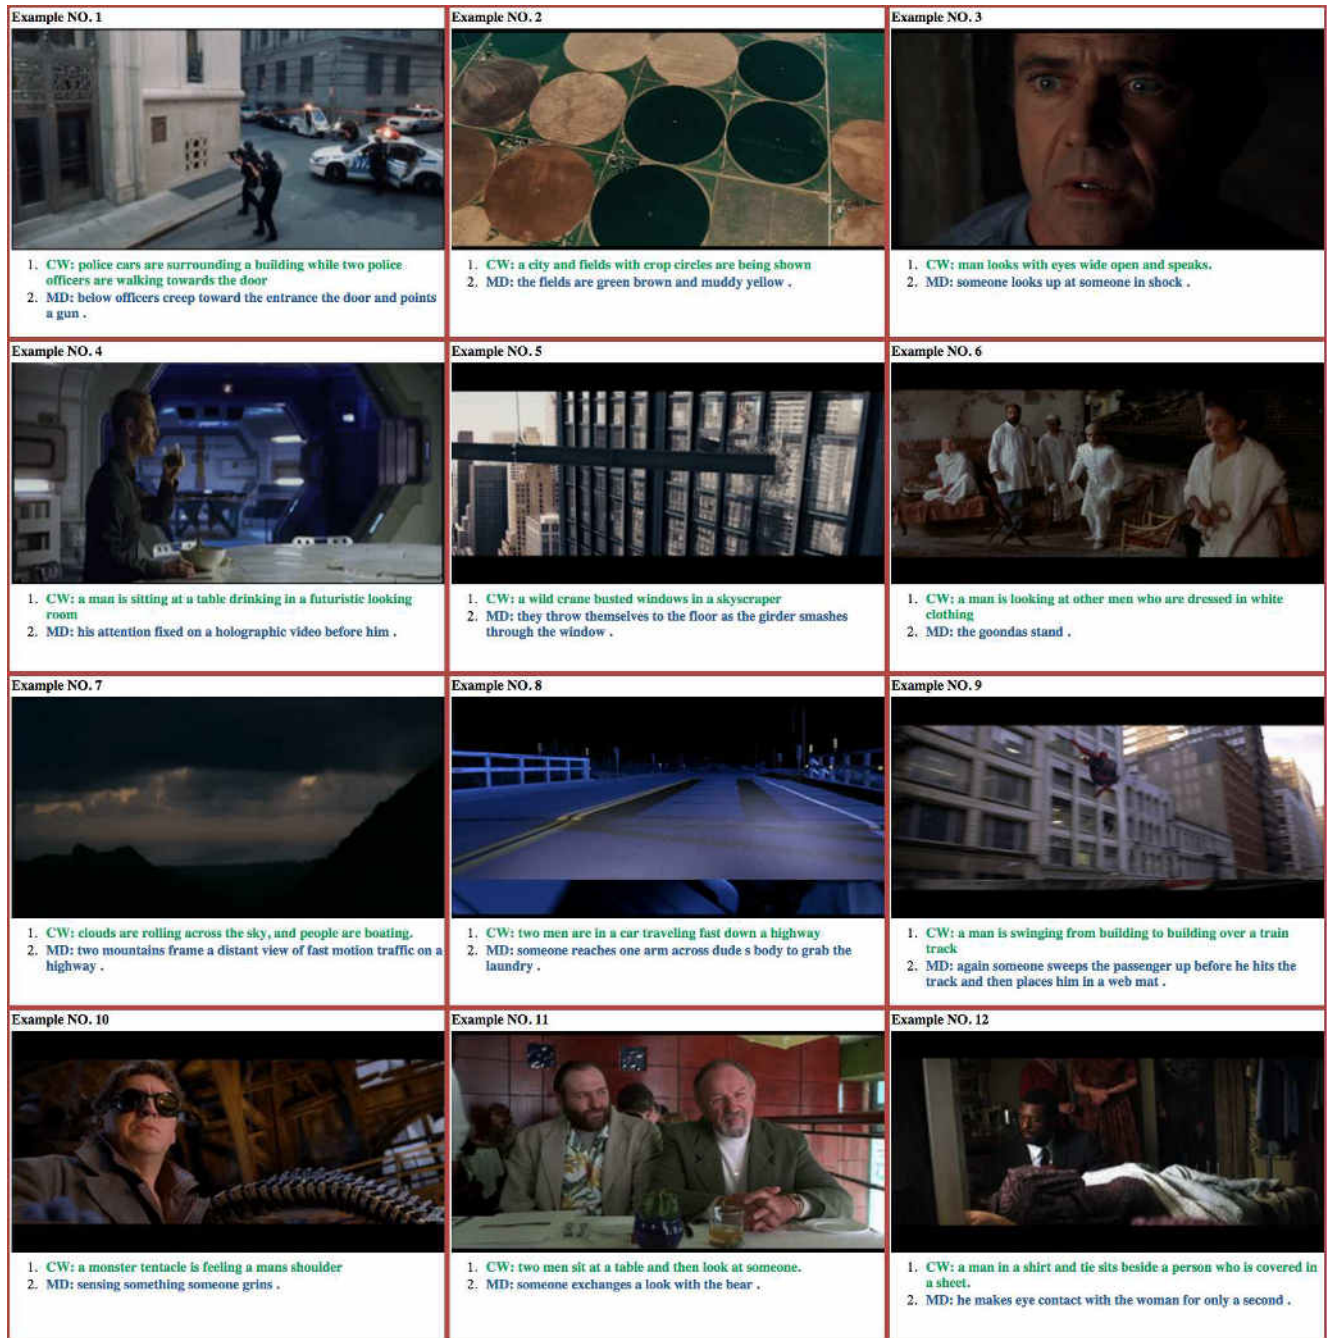 <p>1. CW: a man is sitting at a table drinking in a futuristic looking room<br/>2. MD: his attention fixed on a holographic video before him .</p>                                          | <p>Example NO. 5</p> 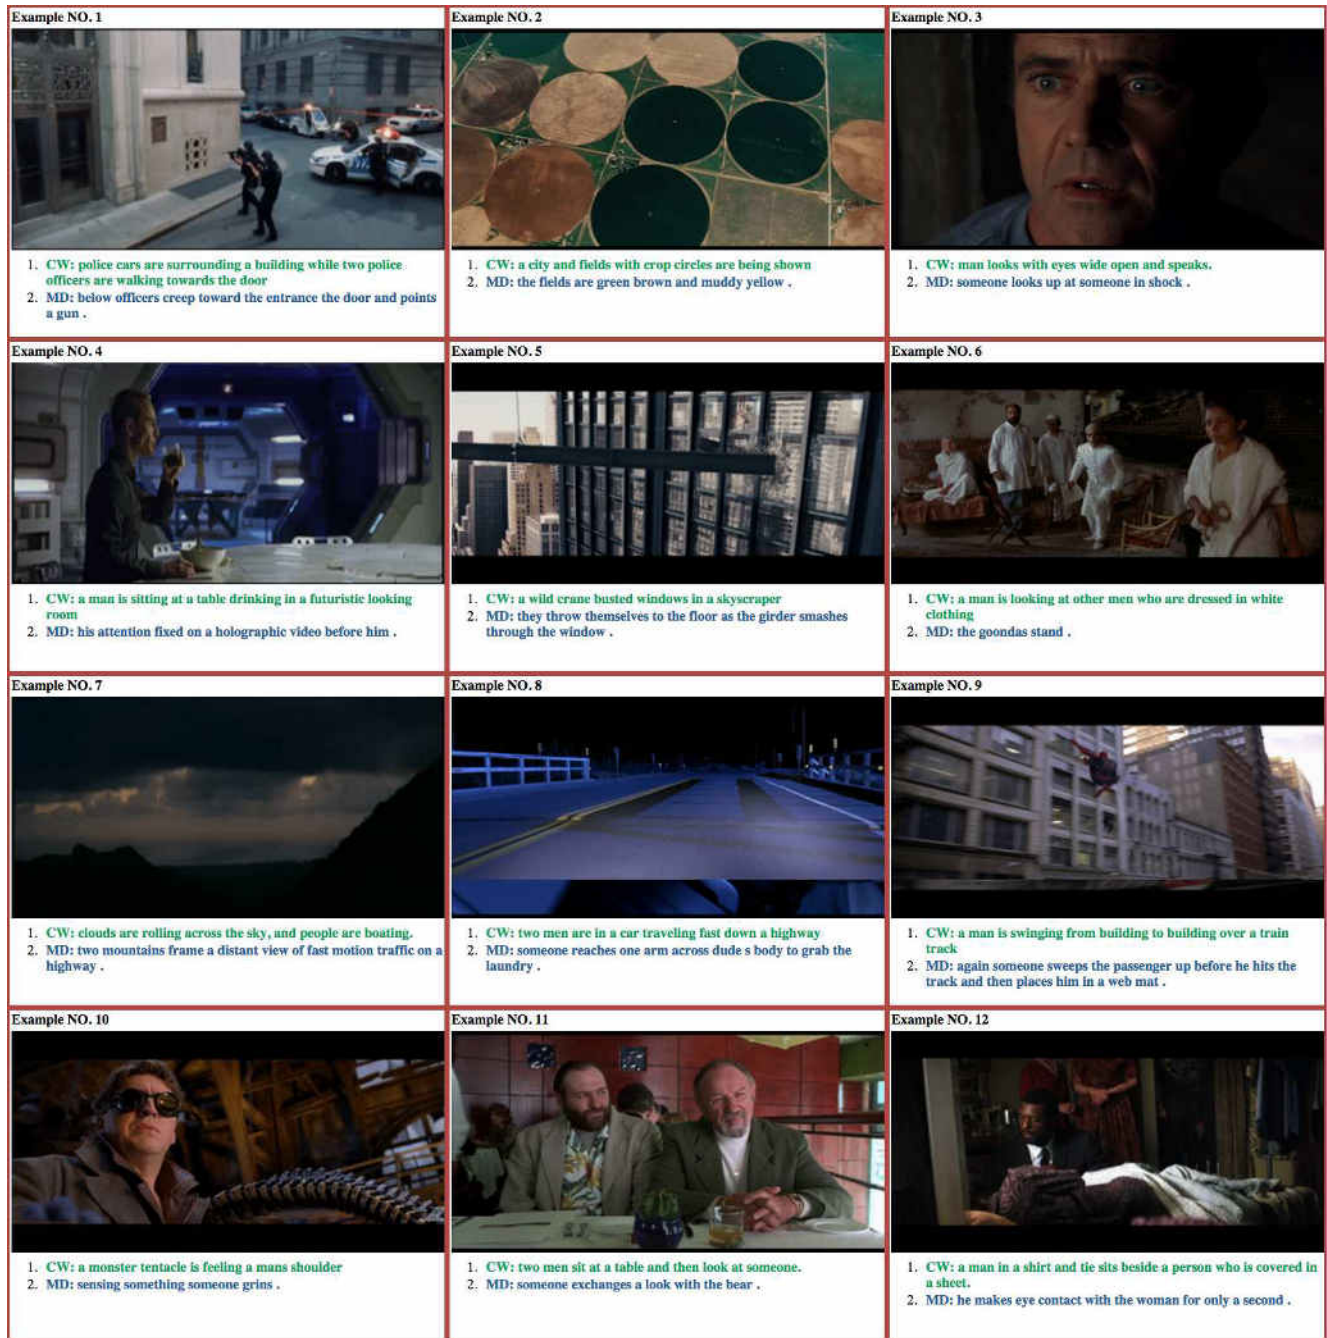 <p>1. CW: a wild crane busted windows in a skyscraper<br/>2. MD: they throw themselves to the floor as the girder smashes through the window .</p> | <p>Example NO. 6</p> 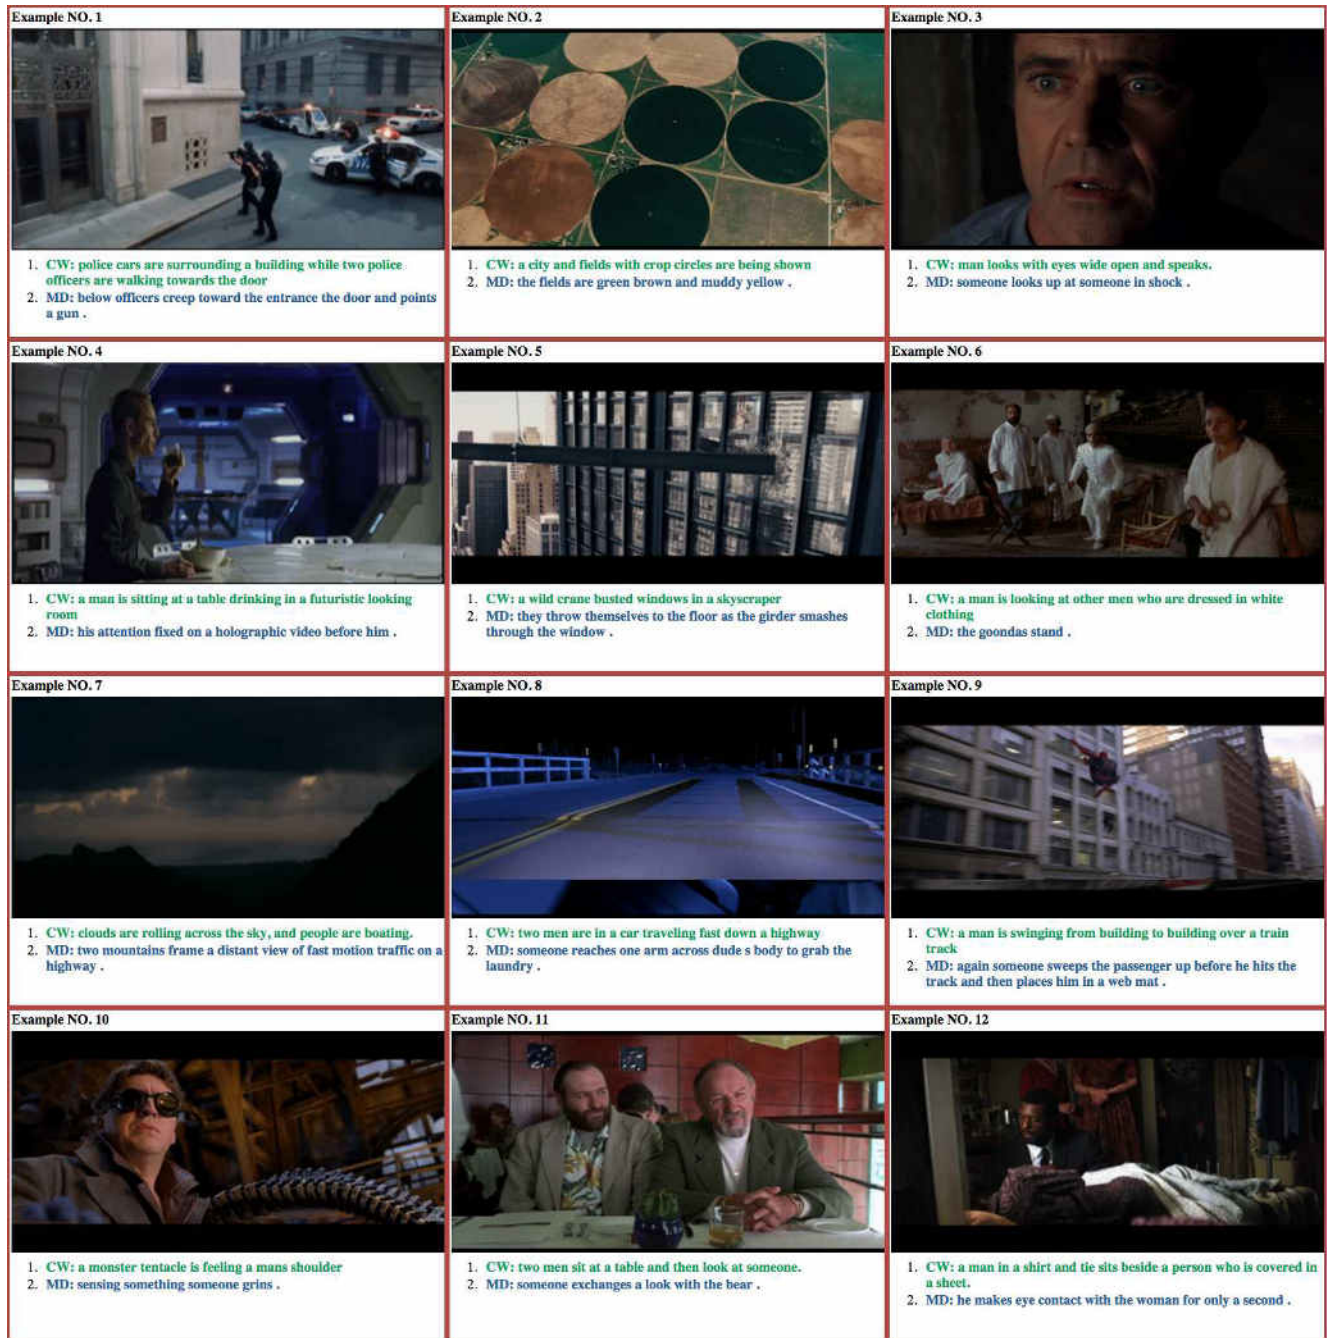 <p>1. CW: a man is looking at other men who are dressed in white clothing<br/>2. MD: the goondas stand .</p>                                                                               |
| <p>Example NO. 7</p> 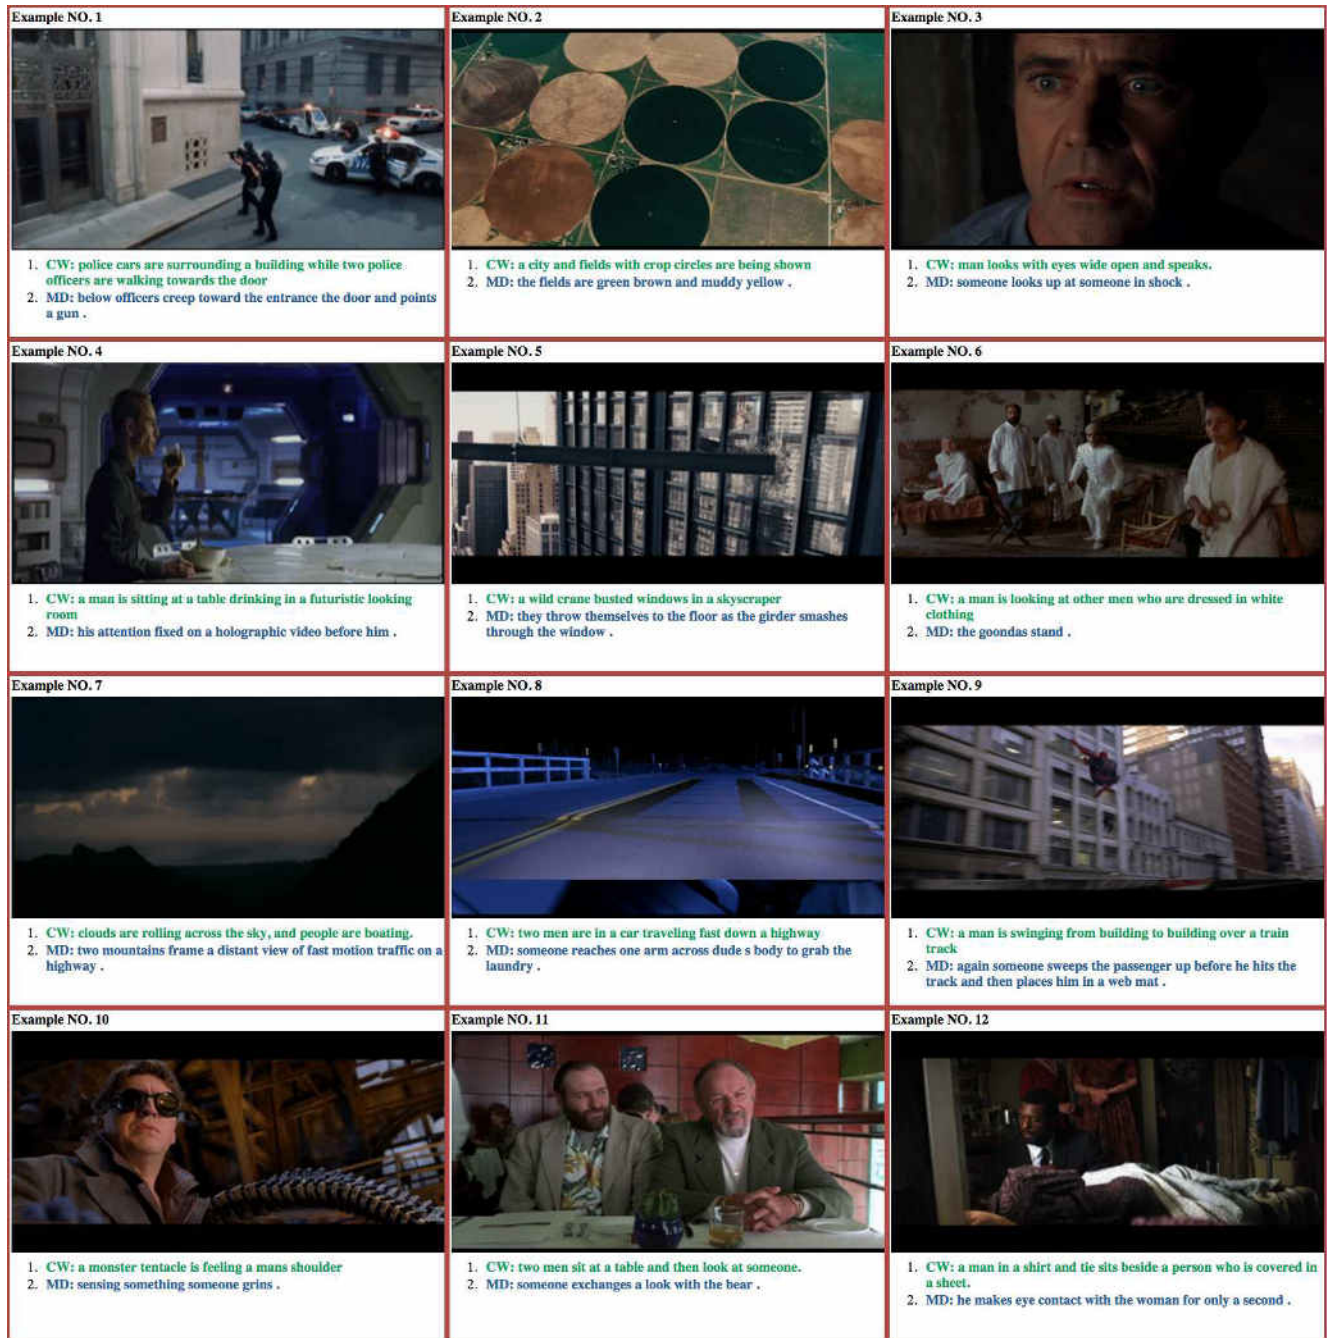 <p>1. CW: clouds are rolling across the sky, and people are boating.<br/>2. MD: two mountains frame a distant view of fast motion traffic on a highway .</p>                               | <p>Example NO. 8</p> 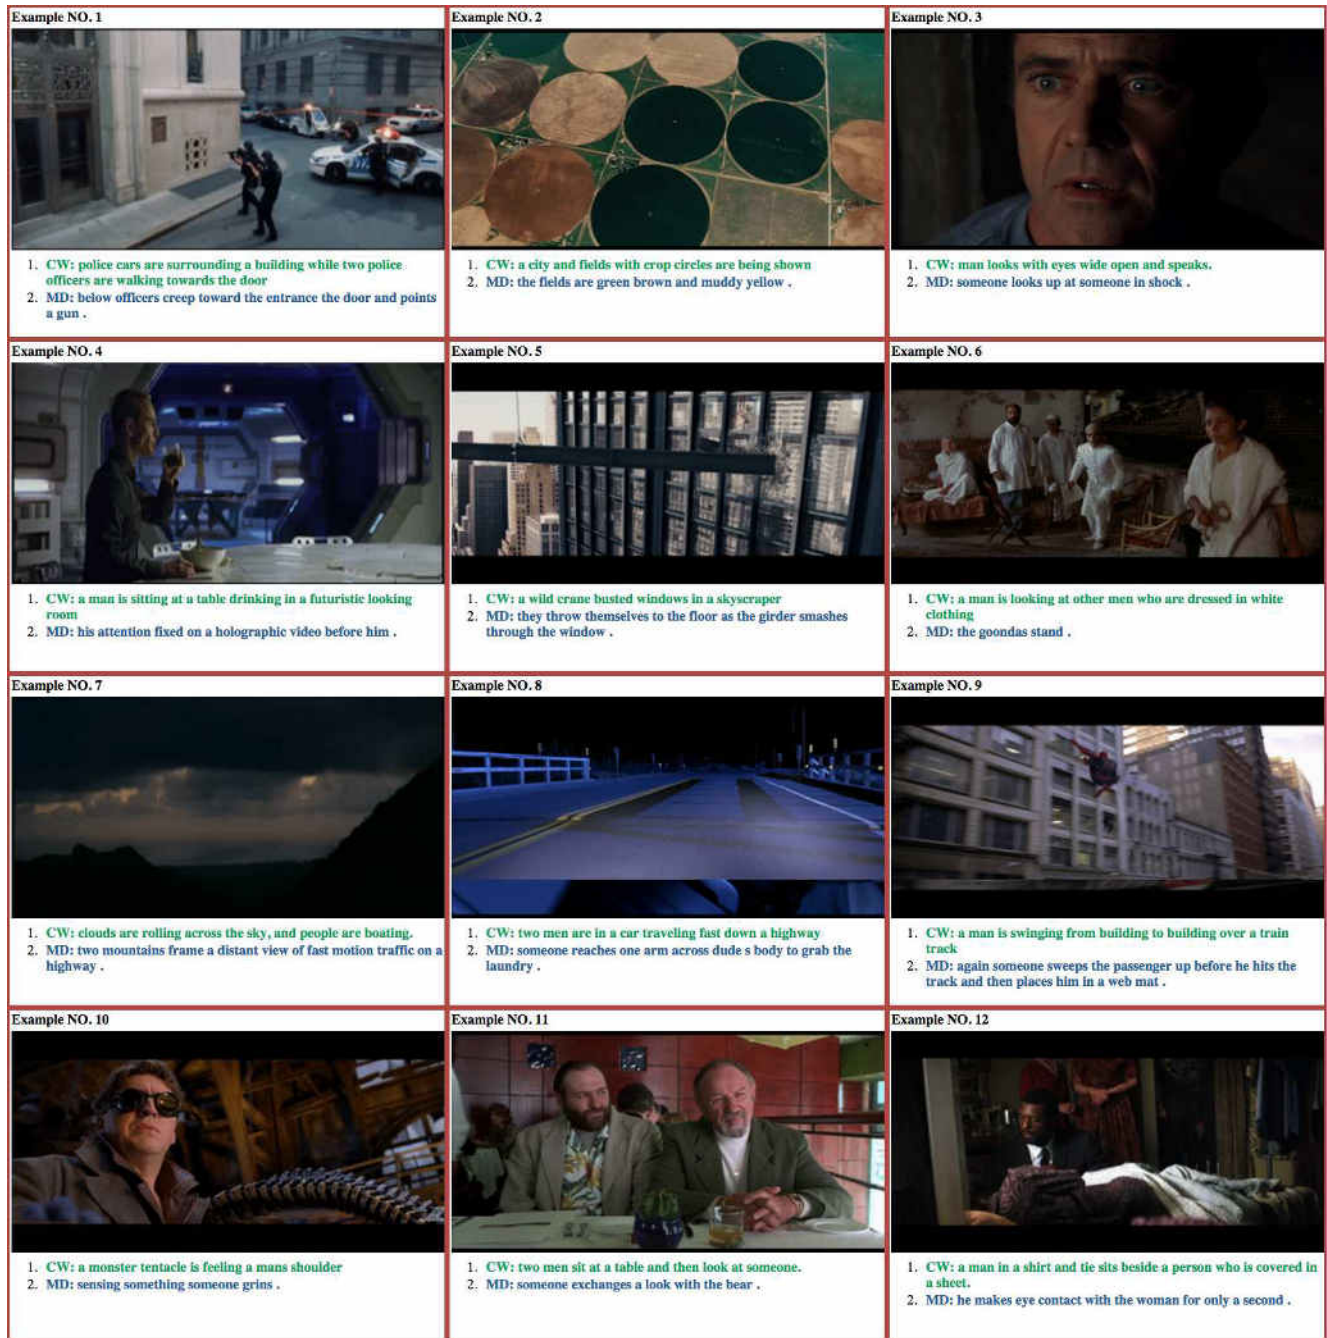 <p>1. CW: two men are in a car traveling fast down a highway<br/>2. MD: someone reaches one arm across dude s body to grab the laundry .</p>      | <p>Example NO. 9</p> 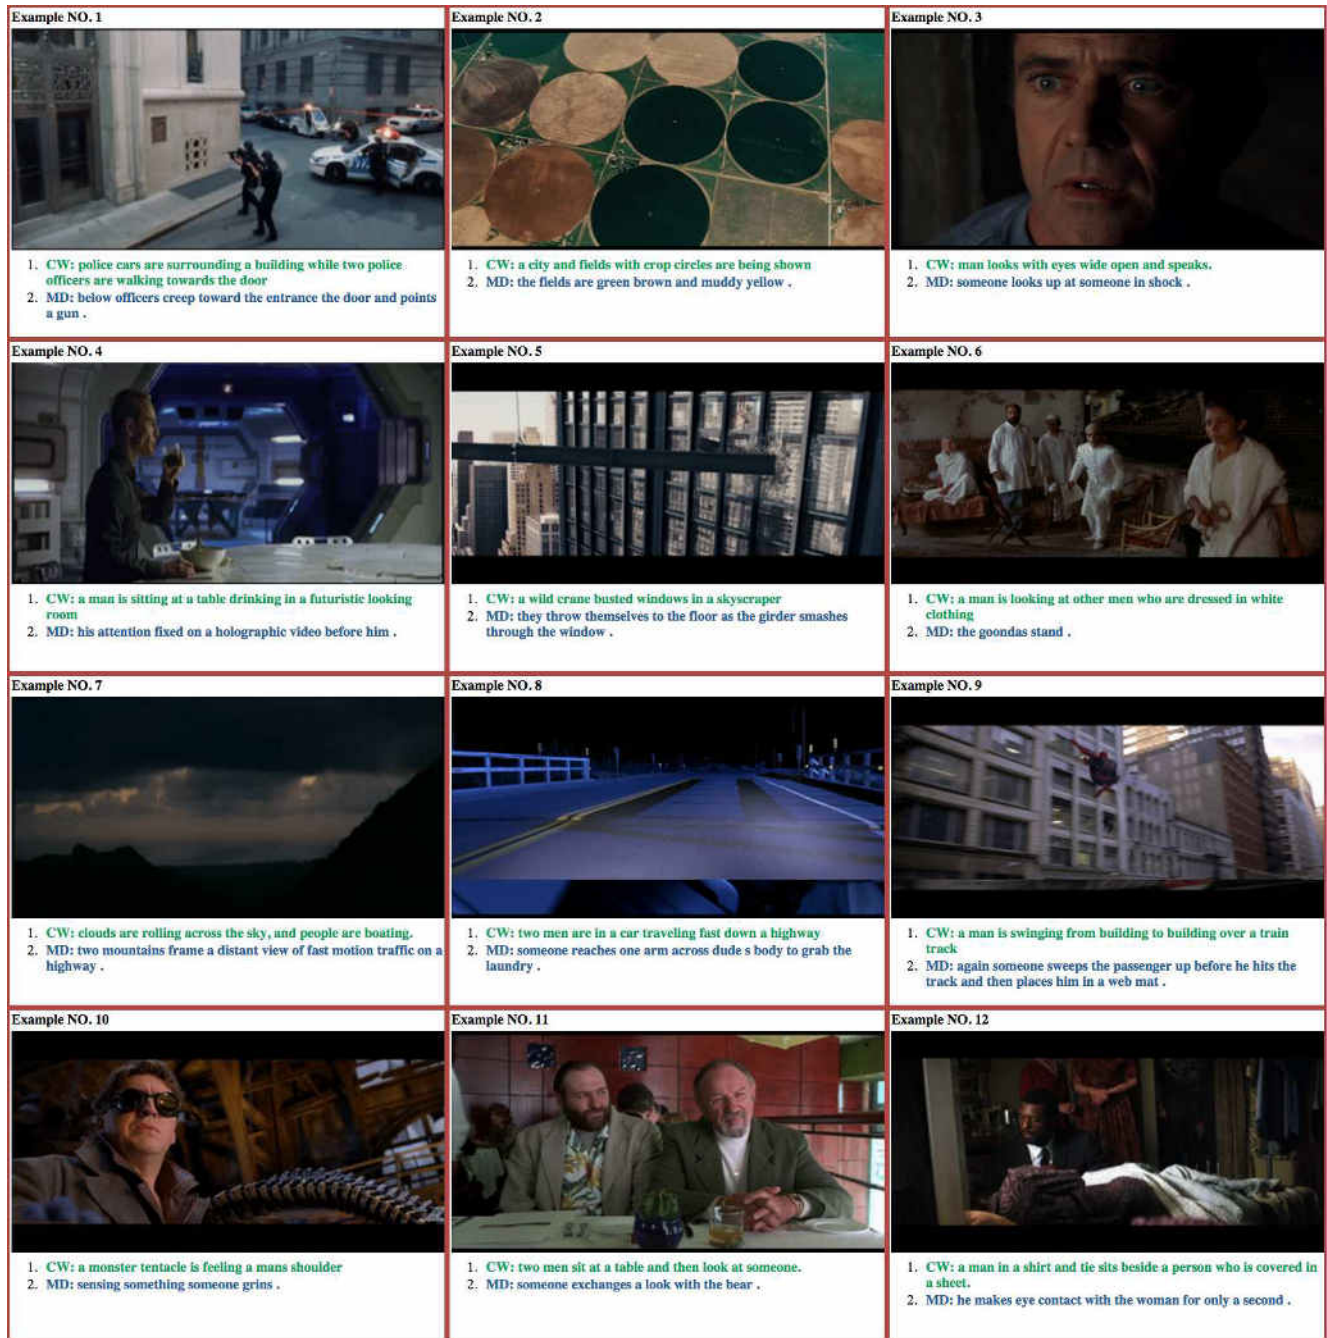 <p>1. CW: a man is swinging from building to building over a train track<br/>2. MD: again someone sweeps the passenger up before he hits the track and then places him in a web mat .</p> |
| <p>Example NO. 10</p> 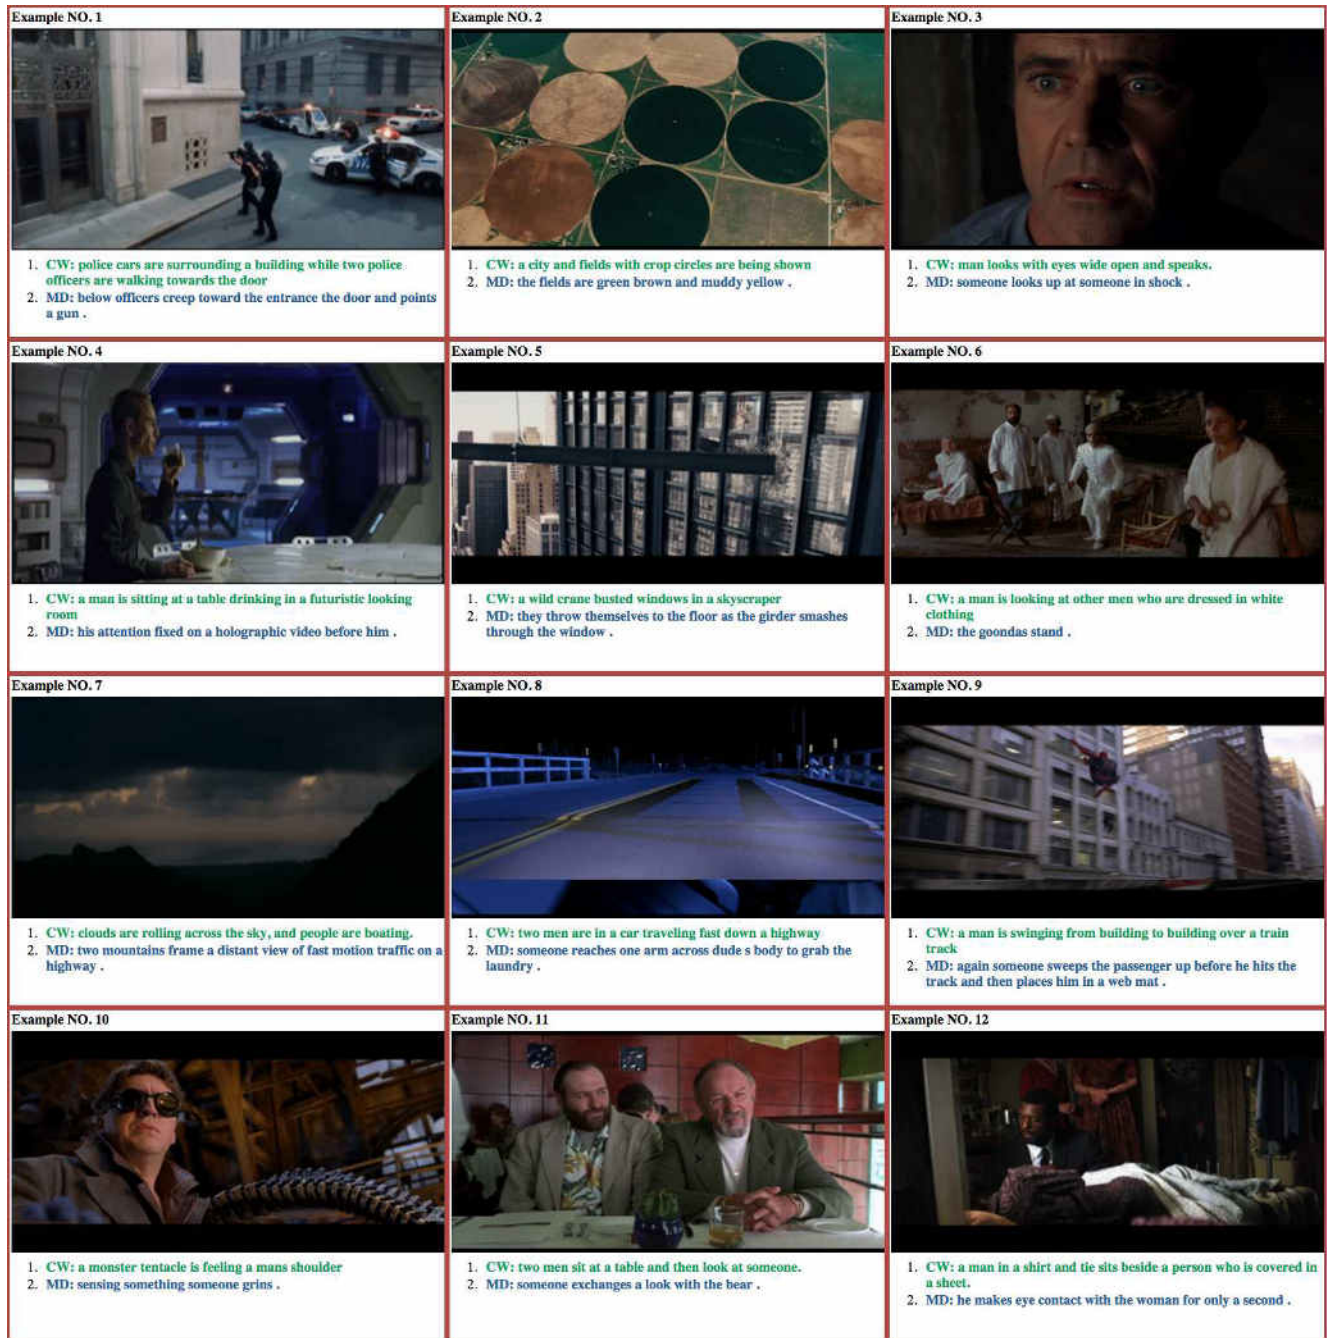 <p>1. CW: a monster tentacle is feeling a mans shoulder<br/>2. MD: sensing something someone grins .</p>                                                                                 | <p>Example NO. 11</p> 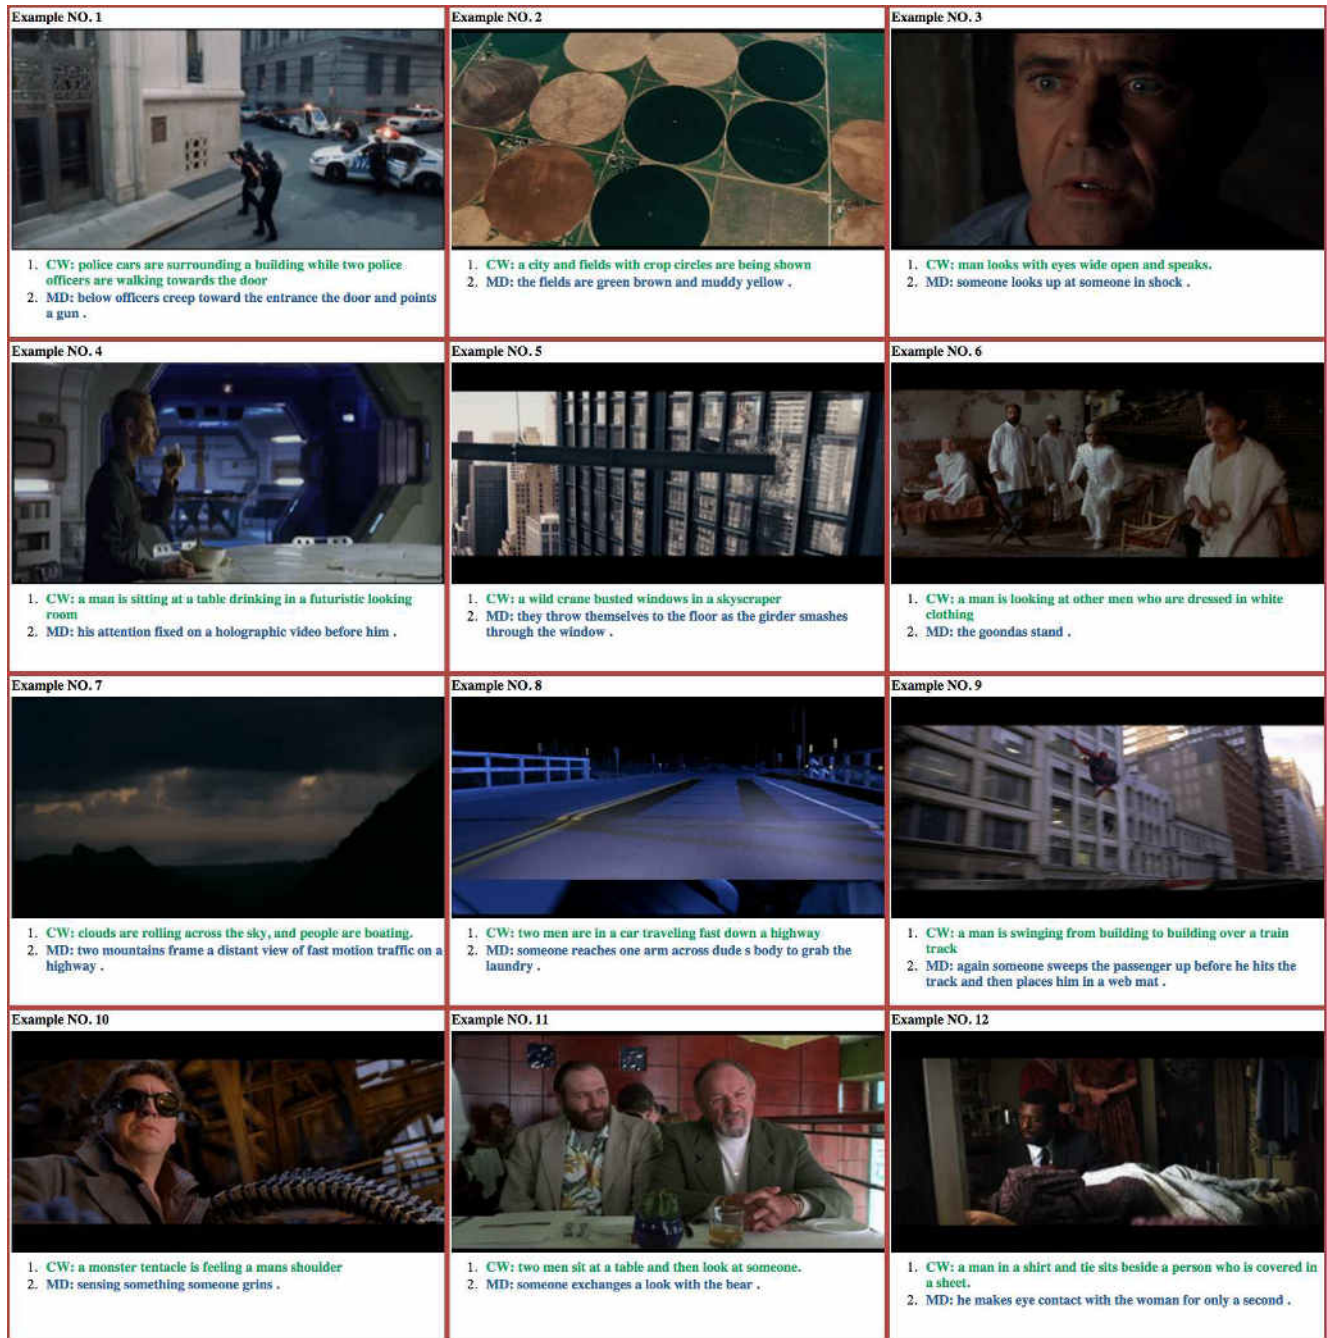 <p>1. CW: two men sit at a table and then look at someone.<br/>2. MD: someone exchanges a look with the bear .</p>                              | <p>Example NO. 12</p> 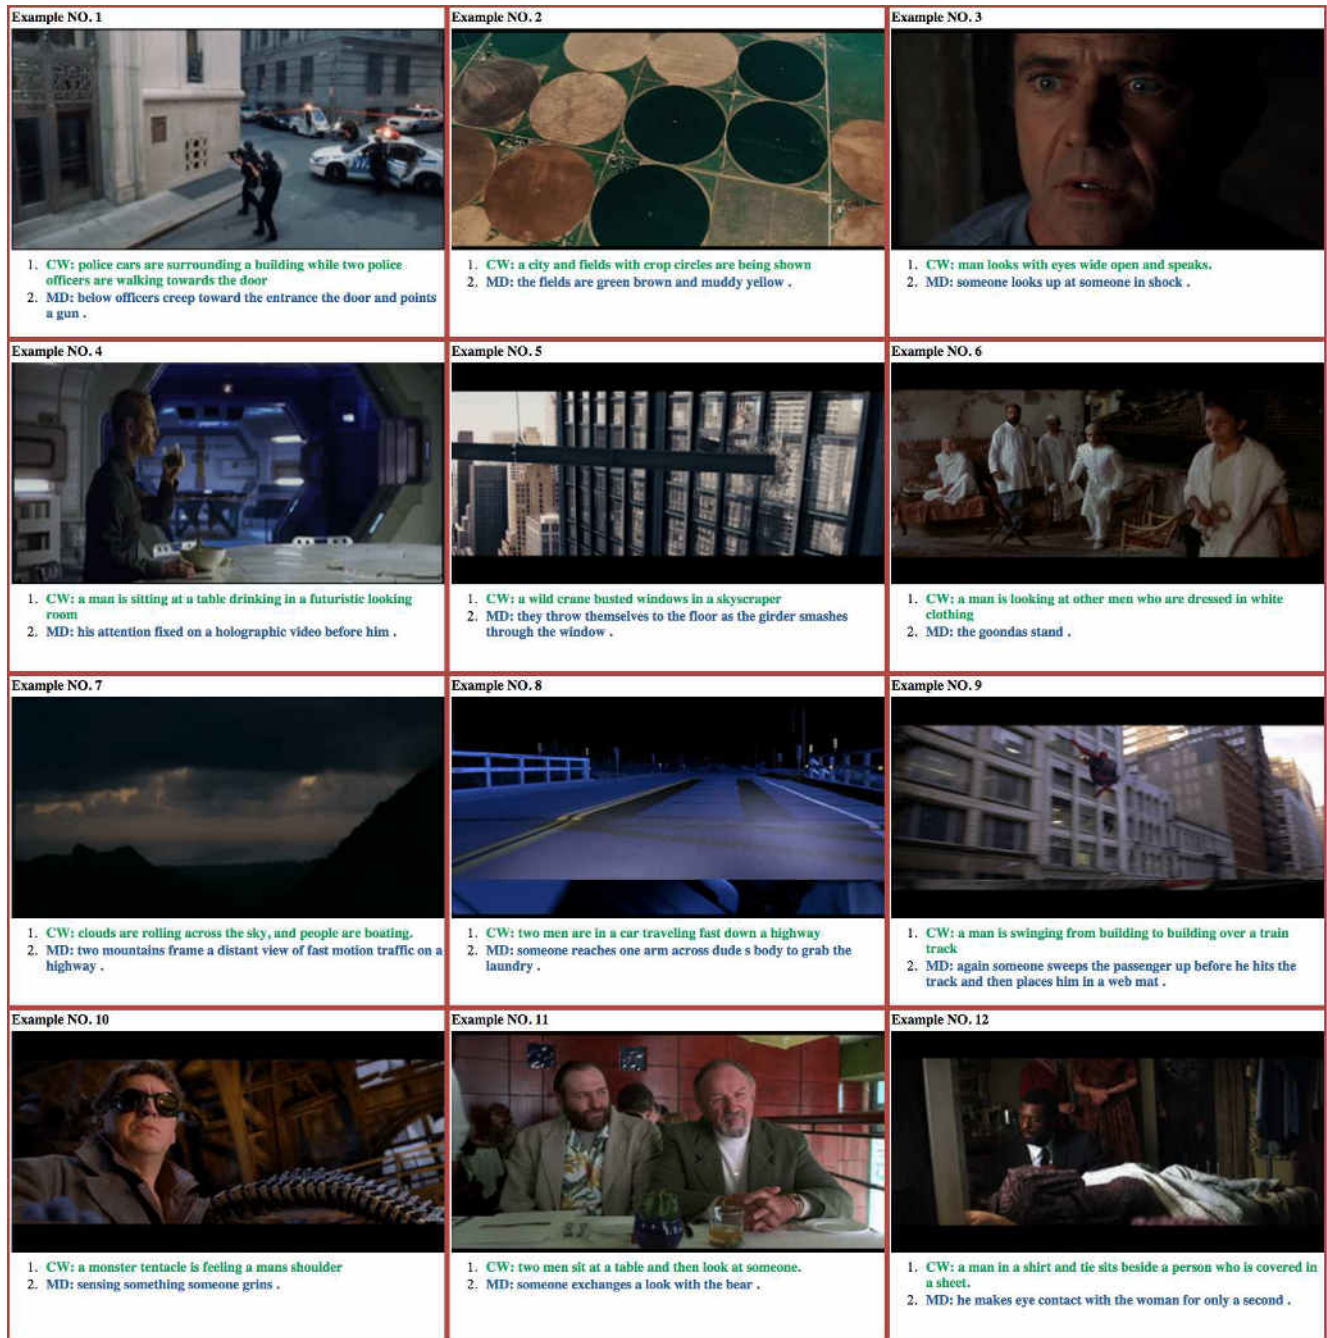 <p>1. CW: a man in a shirt and tie sits beside a person who is covered in a sheet.<br/>2. MD: he makes eye contact with the woman for only a second .</p>                               |

Figure 5: Side-by-side qualitative comparisons of sentences provided in the LSMDC dataset (professionally annotated descriptive video service (DVS) captions) and sentences annotated by the crowd workers. We converted movie clips from the LSMDC dataset into the GIF format and used the same pipeline described in our paper (Section 3) to crowdsource descriptions for the clips. Below each movie clip, we show both the **crowdsourced description (CW)** and the **original description found in the LSMDC dataset (MD)**. We can see that the DVS captions tend to focus on visual content related specifically to the story (e.g., example No.6) or rely on contextual information not actually present within a video clip (e.g., “bear” in example No.11). More examples with better visualization: <https://goo.gl/ZGYIYh>
